# Supplementary material for: NatCat: Weakly Supervised Text Classification with Naturally Annotated Resources
Source: arXiv:2009.14335 source file (2021-09-19)
Supplement: Supplementary file 1 [file supp-main.tex]

%
% File emnlp2020.tex
%
%% Based on the style files for ACL 2020, which were
%% Based on the style files for ACL 2018, NAACL 2018/19, which were
%% Based on the style files for ACL-2015, with some improvements
%%  taken from the NAACL-2016 style
%% Based on the style files for ACL-2014, which were, in turn,
%% based on ACL-2013, ACL-2012, ACL-2011, ACL-2010, ACL-IJCNLP-2009,
%% EACL-2009, IJCNLP-2008...
%% Based on the style files for EACL 2006 by 
%%e.agirre@ehu.es or Sergi.Balari@uab.es
%% and that of ACL 08 by Joakim Nivre and Noah Smith

\documentclass[11pt,a4paper]{article}
\usepackage[hyperref]{emnlp2020}
\usepackage{times}
\usepackage{booktabs}
\usepackage{latexsym}
\usepackage{xspace}
\usepackage{multicol}
\usepackage{multirow}
\usepackage{amsmath}
\usepackage{amssymb}
\usepackage{graphicx}

% This is not strictly necessary, and may be commented out,
% but it will improve the layout of the manuscript,
% and will typically save some space.
\usepackage{microtype}

%\aclfinalcopy % Uncomment this line for the final submission
%\def\aclpaperid{***} %  Enter the acl Paper ID here

%\setlength\titlebox{5cm}
% You can expand the titlebox if you need extra space
% to show all the authors. Please do not make the titlebox
% smaller than 5cm (the original size); we will check this
% in the camera-ready version and ask you to change it back.

\newcommand{\kevin}[1]{\textcolor{blue}{\bf \small [ #1 --KPG]}}
\newcommand{\karl}[1]{\textcolor{brown}{\bf \small [ #1 --Karl]}}

\newcommand{\zewei}[1]{\textcolor{red}{\bf \small [ #1 --Zewei]}}

\newcommand{\natcat}{\textsc{NatCat}\xspace}

\hyphenation{Nat-Cat}
\hyphenation{Cat-Eval}

\renewcommand{\karl}[1]{}
\renewcommand{\kevin}[1]{}
\renewcommand{\zewei}[1]{}

\title{\natcat: Weakly Supervised Text Classification \\with Naturally Annotated Datasets}
%Text and Categories}

\author{}
\author{Zewei Chu$^1$ \ \ \ \ \ \  Karl Stratos$^2$\thanks{~Work done while the author was at Toyota Technological Institute at Chicago.} \ \ \ \ \ \ Kevin Gimpel$^3$ \\
%[1ex]
$^1$University of Chicago, Chicago, IL, 60637, USA\\
$^2$Rutgers University, New Brunswick, NJ, 08901, USA\\
$^3$Toyota Technological Institute at Chicago, Chicago, IL, 60637, USA\\
%[1ex]
{\small
{\tt zeweichu@uchicago.edu},
{\tt karlstratos@gmail.com},
{\tt kgimpel@ttic.edu}
}\\}
\date{}

\begin{document}
\maketitle

\input{supp}

\bibliographystyle{acl_natbib}
\bibliography{anthology,emnlp2020}

\end{document}
